# Supplementary material for: The Summary Loop: Learning to Write Abstractive Summaries Without Examples
Source: arXiv:2105.05361 source file (2021-05-11)
Supplement: Supplementary file 1 [file old_supplemental.tex]

\begin{figure*}[!htbp]

    \begin{framed}
        % \small
        \textbf{Document}: A giant relative of the kangaroo with the face of a rabbit ambled around the Australian outback 100,000 years ago, according to a new study. Instead of hopping around like its modern cousin, it walked upright, one foot in front of the other, like a human. The study, titled "Locomotion in Extinct Giant Kangaroos: Were \textbf{Sthenurines} Hop-Less Monsters?" and published in the journal PlOS One, said some of the creatures grew up to 7 feet tall and weighed up to 550 pounds, making them poor hoppers. "I don't think they could have gotten that large unless they were walking", said Christine Janis, the lead researcher and a professor of ecology and evolutionary biology at Brown University. Members of the now extinct family of \textbf{sthenurine} kangaroos were likely bipedal walkers, the study said, basing its findings on a biomechanical analysis of the bones of \textbf{sthenurines} and other kangaroos. [...]
        
        \textbf{Target Length}: 10 words

        \textbf{Generated Summary}: The study of \textbf{sthenurines} in Australia
        
        \textit{\textbf{Phenomena observed}: New abstractive sentence. Handling of uncommon words (sthenurine). Use of a word not present in article (Australia). }

        \vspace{1.0em}
        \hrule
        \vspace{1.0em}

        \textbf{Document}: A farmer has lost a nine-year legal battle to save the dream home he built without planning permission and hid behind hay bales for four years. Robert Fidler, 66, secretly constructed the mock-Tudor castle complete with battlements and cannons and lived there with his family from 2002. He unveiled it officially in 2006 when he thought he would be able to exploit a legal loophole that prevents enforcement action against a structure if no objections have been made for at least four years. Scroll down for video. Robert Fidler has lost a nine-year legal battle to save the dream home (above) he built in Salfords, Surrey, without planning permission and hid behind hay bales for four years. But the local authority immediately laid siege by refusing to grant retrospective permission. [...]
        
        \textbf{Target Length}: 45 words
        
        \textbf{Generated Summary}: Robert Fidler has lost a nine-year legal battle to save the dream home he built without planning permission and hid behind hay bales for four years. He built the mock-Tudor castle complete with battlements and cannons. He unveiled it officially in 2006.
    
        \textit{\textbf{Phenomena observed:} Swapping sentence subjects for named entity. Sentence simplification, selecting content most relevant for a summary.}
    
        \vspace{1.0em}
    
        \hrule
        \vspace{1.0em}
        
        \textbf{Document}: Desperate migrants from Africa and the Middle East keep heading to Europe, with 978 rescued Friday in the Mediterranean Sea, the Italian Coast Guard said Saturday via Twitter. The migrants were picked up 30 miles off the coast of Libya, \textbf{said European Parliament member Matteo Salvini}, the leader of Italy 's far-right Northern League. In the first three months of 2015, Italy registered more than 10,000 migrants arriving, the International Organization for Migration said, and about 2,000 were rescued at sea during the first weekend of April in the \textbf{Channel of Sicily}. Most migrants recorded this year come from countries in West Africa as well as Somalia and Syria, the IMO said. They use Libya as a country of transit. At least 480 migrants have died while crossing the Mediterranean since the beginning of the year, often because of bad weather and overcrowded vessels used by smugglers, the IMO said. Sometimes the captains and crews abandon the ships, leaving passengers to fend for themselves. [...]
        
        \textbf{Target Length}: 45 words
        
        \textbf{Generated Summary}: The \textbf{IMO} said that migrants were picked up 30 miles off the coast of Libya's far-right Northern League. In the first three months of 2015, Italy registered more than 10,000 migrants arriving at sea. Most migrants were rescued at sea during the first weekend of April in \textbf{the Mediterranean}.
    
        \textit{\textbf{Phenomena observed:} \textcolor{red}{Factual innacuracy}: IMO is confused with Matteo Salvini. Entity swapping: Channel of Sicily is replaced with shorter Mediterranean. Sentence simplifying: long sentence divided into 2 shorter ones.}

        % \textbf{Document}: Three Orthodox rabbis accused of planning and participating in the torture of Jewish men who refused to divorce their wives were convicted Tuesday of conspiring to commit kidnapping. Rabbis Mendel \textbf{Epstein}, 69; Jay Goldstein, 60; and Binyamin \textbf{Stimler}, 39, were found guilty on one count of conspiracy to commit kidnapping in New Jersey federal court. Goldstein and Stimler were also convicted on charges of attempted kidnapping. The rabbis were part of a ring accused of accepting tens of thousands of dollars to orchestrate the kidnappings of Jewish husbands to persuade them through torture involving electric cattle prods and screwdrivers to grant " gets, " a document that Jewish law requires a husband to present to his wife in order to be issued a divorce, court papers said. The men were arrested in October 2013 following an FBI sting operation that ended with Goldstein, Stimler and six other men with ski masks, surgical blades and a 30-foot nylon rope in a warehouse in Middlesex County, New Jersey. [...]
        
        % \textbf{Target Length}: 45 words
        
        % \textbf{Generated Summary}: Rabbi \texbf{Epstein and Stimler} were convicted on charges of conspiracy to commit kidnapping in New Jersey federal court. Goldstein and Stimler were also convicted on charges of attempted kidnapping. Rabbis were part of a ring accused of kidnapping in New Jersey.
    
        % \textit{\textbf{Phenomena observed:} Merging and simplification of entities (removing first name), it however misses 1 of the three Rabbi. Simplification of the third sentence.}

    \end{framed}

    \caption{Hand-picked examples of article, summary pairs generated by the unsupervised Summary Loop models for a given target length. For each, we list the summarization phenomena we observe in the summary. }
    \label{fig:extra_examples}
\end{figure*}
